# Supplementary material for: LoSh: Long-Short Text Joint Prediction Network for Referring Video Object Segmentation
Source: arXiv:2306.08736 source file (2024-04-02)
Supplement: Supplementary file 1 [file X_suppl.tex]

%\clearpage
\setcounter{page}{1}
\maketitlesupplementary
\begin{appendix}

\emph{In this supplementary material, we provide 1) quantitative comparisons between LoSh and other methods on the JHMDB-Sentences dataset; 2) additional ablation studies for LoSh-M and LoSh-S; 
%3) quantitative results of the proposed method built upon an alternative baseline; 
3) additional qualitative results of mask predictions across frames.  The experimental setup follows the default setting in the main body of our paper.}

\begin{table}
\centering
\footnotesize
\begin{tabular}{c|c|ccc}
\hline
{Method} & {\centering Backbone}  &  O-IoU & M-IoU & mAP  \\
 % &  &  O-IoU & M-IoU & mAP \\
\hline\hline
Hu \etal \cite{huetal} & VGG-16  & 54.6 & 52.8 & 17.8 \\
Gavrilyuk \etal \cite{firstRVOS} &  I3D  & 54.1 & 54.2 & 23.3\\
CMPC-V~\cite{CMPC} & I3D  & 61.6 & 61.7 & 34.2  \\
ClawCraneNet~\cite{clawcranenet} & ResNet-50/101  & 64.4 & 65.6 & -  \\
ReferFormer~\cite{ReferFormer} & Video-Swin-T  & 71.9 & 71.0 & 42.2  \\
ReferFormer~\cite{ReferFormer} & Video-Swin-B  & 73.0 & 71.8 & 43.7 \\

\hline

MTTR ${\left(w = 8\right)}$~\cite{MTTR} & Video-Swin-T  & 67.4 & 67.9 & 36.6 \\
\rowcolor{mygray}
\textbf{LoSh-M ${\left(w = 8\right)}$} & Video-Swin-T  & \textbf{70.8} & \textbf{70.4} & \textbf{39.0} \\
\hline
SgMg$\left(w=5\right)$~\cite{SgMg} & Video-Swin-T & 72.8& 71.7 &44.4 \\
\rowcolor{mygray}
\textbf{LoSh-S$\left(w=5\right)$} & Video-Swin-T& \textbf{73.6}& \textbf{72.5} &\textbf{45.0} \\
SgMg$\left(w=5\right)$~\cite{SgMg} & Video-Swin-B & 73.7& 72.5 &45.0 \\
\rowcolor{mygray}
\textbf{LoSh-S$\left(w=5\right)$} & Video-Swin-B& \textbf{74.5}& \textbf{73.4} &\textbf{45.7} \\
\hline
\end{tabular}

\caption{Quantitative comparison with state of the art on  JHMDB-Sentences~\cite{firstRVOS}. O-IoU and M-IoU represent Overall IoU and Mean IoU. The number of input frames $w$ follows the implementation details of~\cite{MTTR,SgMg}.
}
\vspace{-6pt}
\label{tab:SOTAcomparison_on_JHMDB}
\end{table}

\section{Additional quantitative comparisons with state of the art on the JHMDB-Sentences}
To further show the generalizability of our method, we follow~\cite{MTTR, ReferFormer, SgMg} to evaluate the trained LoSh-M and LoSh-S from the A2D-Sentences onto the JHMDB-Sentences without fine-tuning. As shown in Tab.~\ref{tab:SOTAcomparison_on_JHMDB}, LoSh-M and LoSh-S gain massive improvements on all metrics compared to their counterpart baselines (\eg, +2.4 mAP, +3.4\% Overall IoU and +2.5\% Mean IoU when comparing between LoSh-M and MTTR). Furthermore, LoSh-S with Video-Swin-B yields highest results amongst all.

\section{Additional ablation studies on LoSh-M}

{For a fair comparison, we train baseline MTTR~\cite{MTTR} using original long expressions and our generated short ones with their corresponding GTs (Baseline w/ Sh in Tab.~\ref{tab:Ablation for long short}). It shows a relatively marginal increase of +0.6 mAP on A2D-Sentences. While our LoSh-M, by adding interactions between long and short expressions, achieves a noteworthy improvement of +3.1 mAP.} We also provide more ablation studies on LoSh-M in terms of the number of input frames and object queries.
 
\noindent
\textbf{Number of input frames $w$.} We study the effect of the number of input frames on LoSh-M in Tab.~\ref{tab:Ablation for w}. Generally, a larger number of input frames helps the model better extract motion information across frames. Note that when $w=1$, the forward-backward visual consistency loss is deprecated since we can not generate optical flow from only one input frame. When changing $w$ from 1 to 8,  we observe an mAP gain of 4.0 and a Mean IoU gain of 3.1\%. Yet, when $w =12$, the performance slightly drops; we suspect that when the input video gets long, the content becomes complex and irrelevant information is more likely to be included.

\begin{table}
\begin{center}
\begin{tabular}{c|cc|c}
\hline
\multirow{2}{*}{Method} & \multicolumn{2}{c|}{IoU} & \multirow{2}{*}{mAP}  \\ \cline{2-3}
 & Overall& Mean& \\
\hline\hline
Baseline & 70.2 & 61.8 & 44.7\\
Baseline w/ Sh & 72.3 & 63.5 &45.4 \\
\textbf{Losh-M (Ours)} & \textbf{72.9} &\textbf{64.9} & \textbf{47.8}\\

\hline
\end{tabular}
\end{center}
\setlength{\abovecaptionskip}{-0.3cm}
\setlength{\belowcaptionskip}{-0.2cm}
\caption{Ablation study for long-short text joint prediction.}
\vspace{-6pt}
\label{tab:Ablation for long short}
\end{table}

\begin{table}
\begin{center}
\begin{tabular}{c|cc|c}
\hline
\multirow{2}{*}{$w$} & \multicolumn{2}{c|}{IoU} & \multirow{2}{*}{mAP}  \\ \cline{2-3}
 & Overall& Mean& \\
\hline\hline
1 &70.3 & 61.8 & 43.8 \\
5 &72.3 & 64.5 & 46.9 \\
\textbf{8} & \textbf{72.9} &\textbf{64.9} & \textbf{47.8}\\
12 & 72.4 & 64.5 & 47.0 \\

\hline
\end{tabular}
\end{center}
\setlength{\abovecaptionskip}{-0.3cm}
\setlength{\belowcaptionskip}{-0.2cm}
\caption{ Ablation study for the number of input frames.}
\label{tab:Ablation for w}
\end{table}

\begin{table}
\begin{center}
\begin{tabular}{c|cc|c}
\hline
\multirow{2}{*}{$N$} & \multicolumn{2}{c|}{IoU} & \multirow{2}{*}{mAP}  \\ \cline{2-3}
 & Overall& Mean& \\
\hline\hline
20 & 72.6 & 64.2 & 45.8\\
\textbf{50} & \textbf{72.9} &\textbf{64.9} & \textbf{47.8}\\
80 & 72.4 & 64.2 & 45.5\\

\hline
\end{tabular}
\end{center}
\setlength{\abovecaptionskip}{-0.3cm}
\setlength{\belowcaptionskip}{-0.2cm}
\caption{ Ablation study for the number of object queries.}
\label{tab:Ablation for N}
\end{table}

\noindent
\textbf{Number of object queries $N$.} We study the effect of the number of object queries on LoSh-M  in Tab.~\ref{tab:Ablation for N}. Given our default setting $N=50$, LoSh-M gains the best performance. The performance drops with a smaller $N$ as the smaller set of object queries might not be diverse enough to cover the target instance in the video. 
%More object queries enable the model to generate the final mask prediction from a wide range of instance candidates. 
%This helps the model better handle sophisticated scenes. 
However, a larger $N$ also ends up with some performance drop. During training, only the object query which is matched with the ground-truth instance is trained while others are ignored. This means that many object queries cannot be fully trained, resulting into sub-optimal performance.

%\renewcommand{\thetable}{A.1}
% \begin{table*}[t]
% \begin{center}
% \small
% \begin{tabular}{c|ccc|ccc|ccc|ccc}
% \hline
% \multirow{2}{*}{Method} &\multicolumn{3}{c|}{A2D-Sentences} &\multicolumn{3}{c|}{JHMDB-Sentences} &\multicolumn{3}{c|}{Refer-YouTube-VOS} &\multicolumn{3}{c}{Refer-DAVIS17}  \\ \cline{2-13} 
%  & O-IoU & M-IoU & mAP  & O-IoU & M-IoU & mAP & {$\mathcal{J} \& \mathcal{F}$} & {$\mathcal{J}$} &  {$\mathcal{F}$} & {$\mathcal{J} \& \mathcal{F}$} & {$\mathcal{J}$} &  {$\mathcal{F}$} \\

% \hline\hline
% ReferFormer~\cite{ReferFormer} & 78.6& 70.3& 55.0 &73.0 &71.8 &43.7 & 62.9 & 61.3 & 64.6 & 61.1& 58.1& 64.1 \\
% \textbf{LoSh-R (ours)} & \textbf{79.9}& \textbf{72.8}& \textbf{56.7} & \textbf{74.2}& \textbf{72.7}& \textbf{45.1}& \textbf{64.4} &\textbf{62.7} & \textbf{66.2}& \textbf{62.6} &\textbf{59.6} & \textbf{65.5} \\

% \hline
% \end{tabular}
% \end{center}
% \setlength{\abovecaptionskip}{-0.3cm}
% \setlength{\belowcaptionskip}{0cm}
% \caption{Quantitative comparison between ReferFormer~\cite{ReferFormer} and LoSh-R on four RVOS datasets. }
% \vspace{-4pt}
% \label{tab:comparison_LoShR}
% \end{table*}

\begin{table}
\begin{center}
\begin{tabular}{c|cc|c}
\hline
\multirow{2}{*}{Method} & \multicolumn{2}{c|}{IoU} & \multirow{2}{*}{mAP}  \\ \cline{2-3}
 & Overall& Mean& \\
\hline\hline

LoSh-S w/o Sh & 78.5 & 70.8 & 56.5\\
LoSh-S w/o $\mathcal L_{lsi}$ & 78.7 & 71.0 & 56.8\\
LoSh-S w/o CA  & 78.9 & 71.3 &  57.2\\
LoSh-S w/o $\mathcal{L}_{fbc}$ & 79.0 & 71.3  & 57.3 \\
\textbf{LoSh-S (Ours)} & \textbf{79.3}& \textbf{71.6}& \textbf{57.6}\\

\hline
\end{tabular}
\end{center}
\setlength{\abovecaptionskip}{-0.3cm}
\setlength{\belowcaptionskip}{-0.2cm}
\caption{ Ablation study for the components in LoSh-S.}
\vspace{-6pt}
\label{tab:Ablation components}
\end{table}

\begin{figure*}
\begin{center}
\includegraphics[width=0.9\linewidth]
% {Figure2_Appendix.png}
{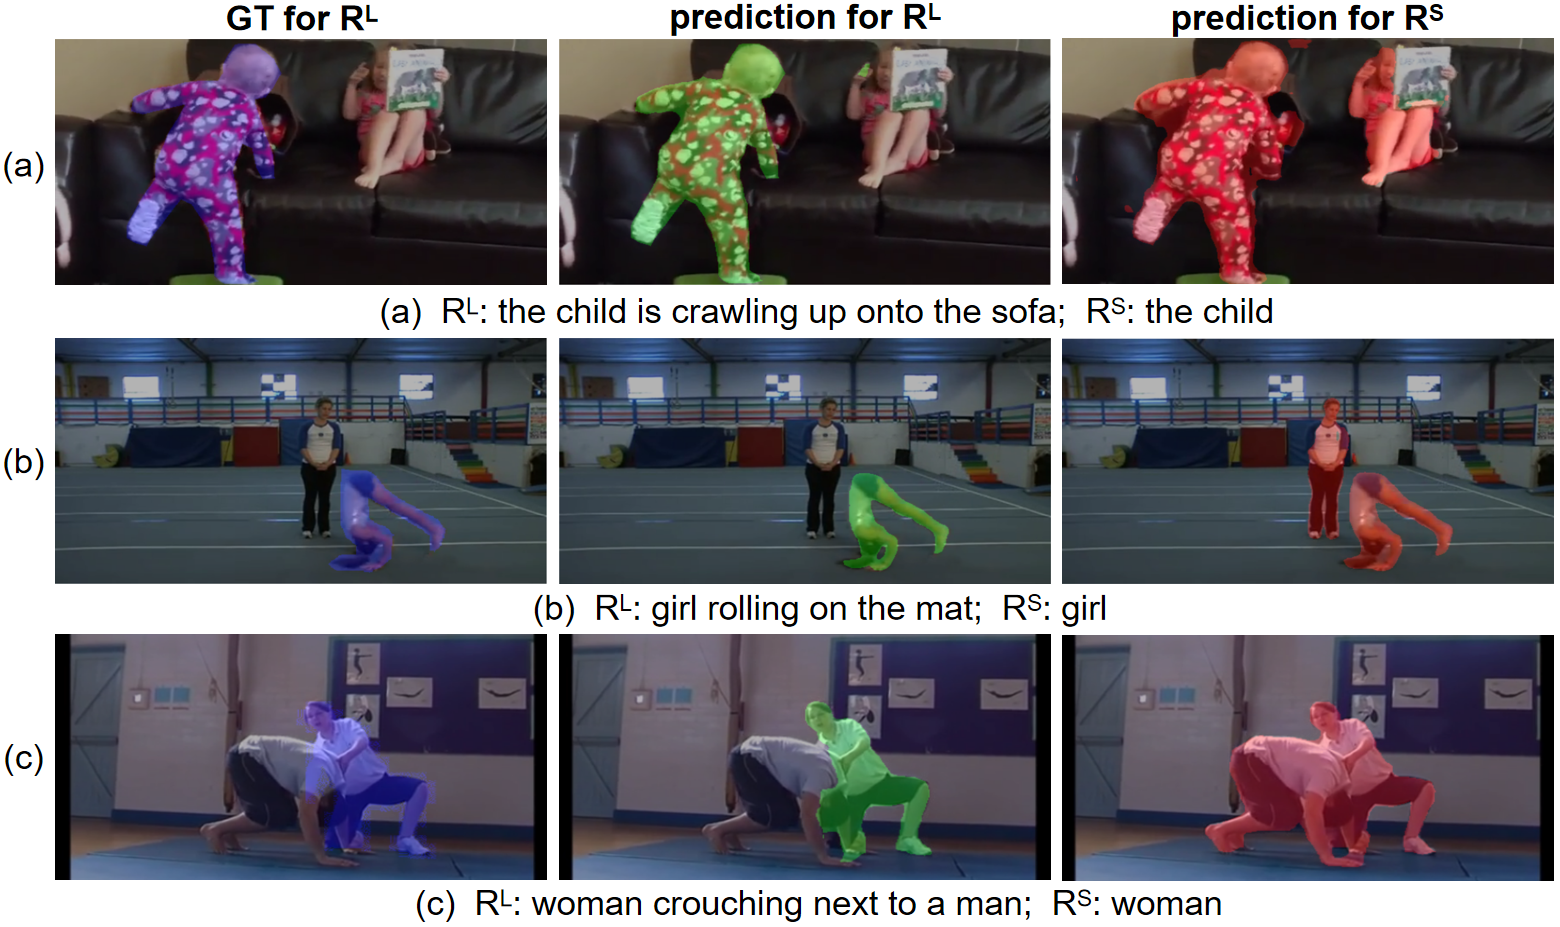}
\setlength{\abovecaptionskip}{-0.3cm}
\setlength{\belowcaptionskip}{-0.2cm}
\end{center}
   \caption{Qualitative results of  mask predictions from LoSh using long and short text expressions, respectively. The three columns from left to right are ground truth, predictions for the long text expressions ($R^L$), and the short expressions ($R^S$), respectively. The long and short text expressions, $R^L$ and $R^S$,  are written below each row.}
   %\miaojing{font! and ground truth!}\linfeng{As our discussion, I don't increase the column for gt.  I have bolded the column title and aligned the text rows on the left.}}
   \vspace{-6pt}
\label{fig:visualization_appendix}
\end{figure*}

\begin{figure*}
\begin{center}
\includegraphics[width=0.9\linewidth]
{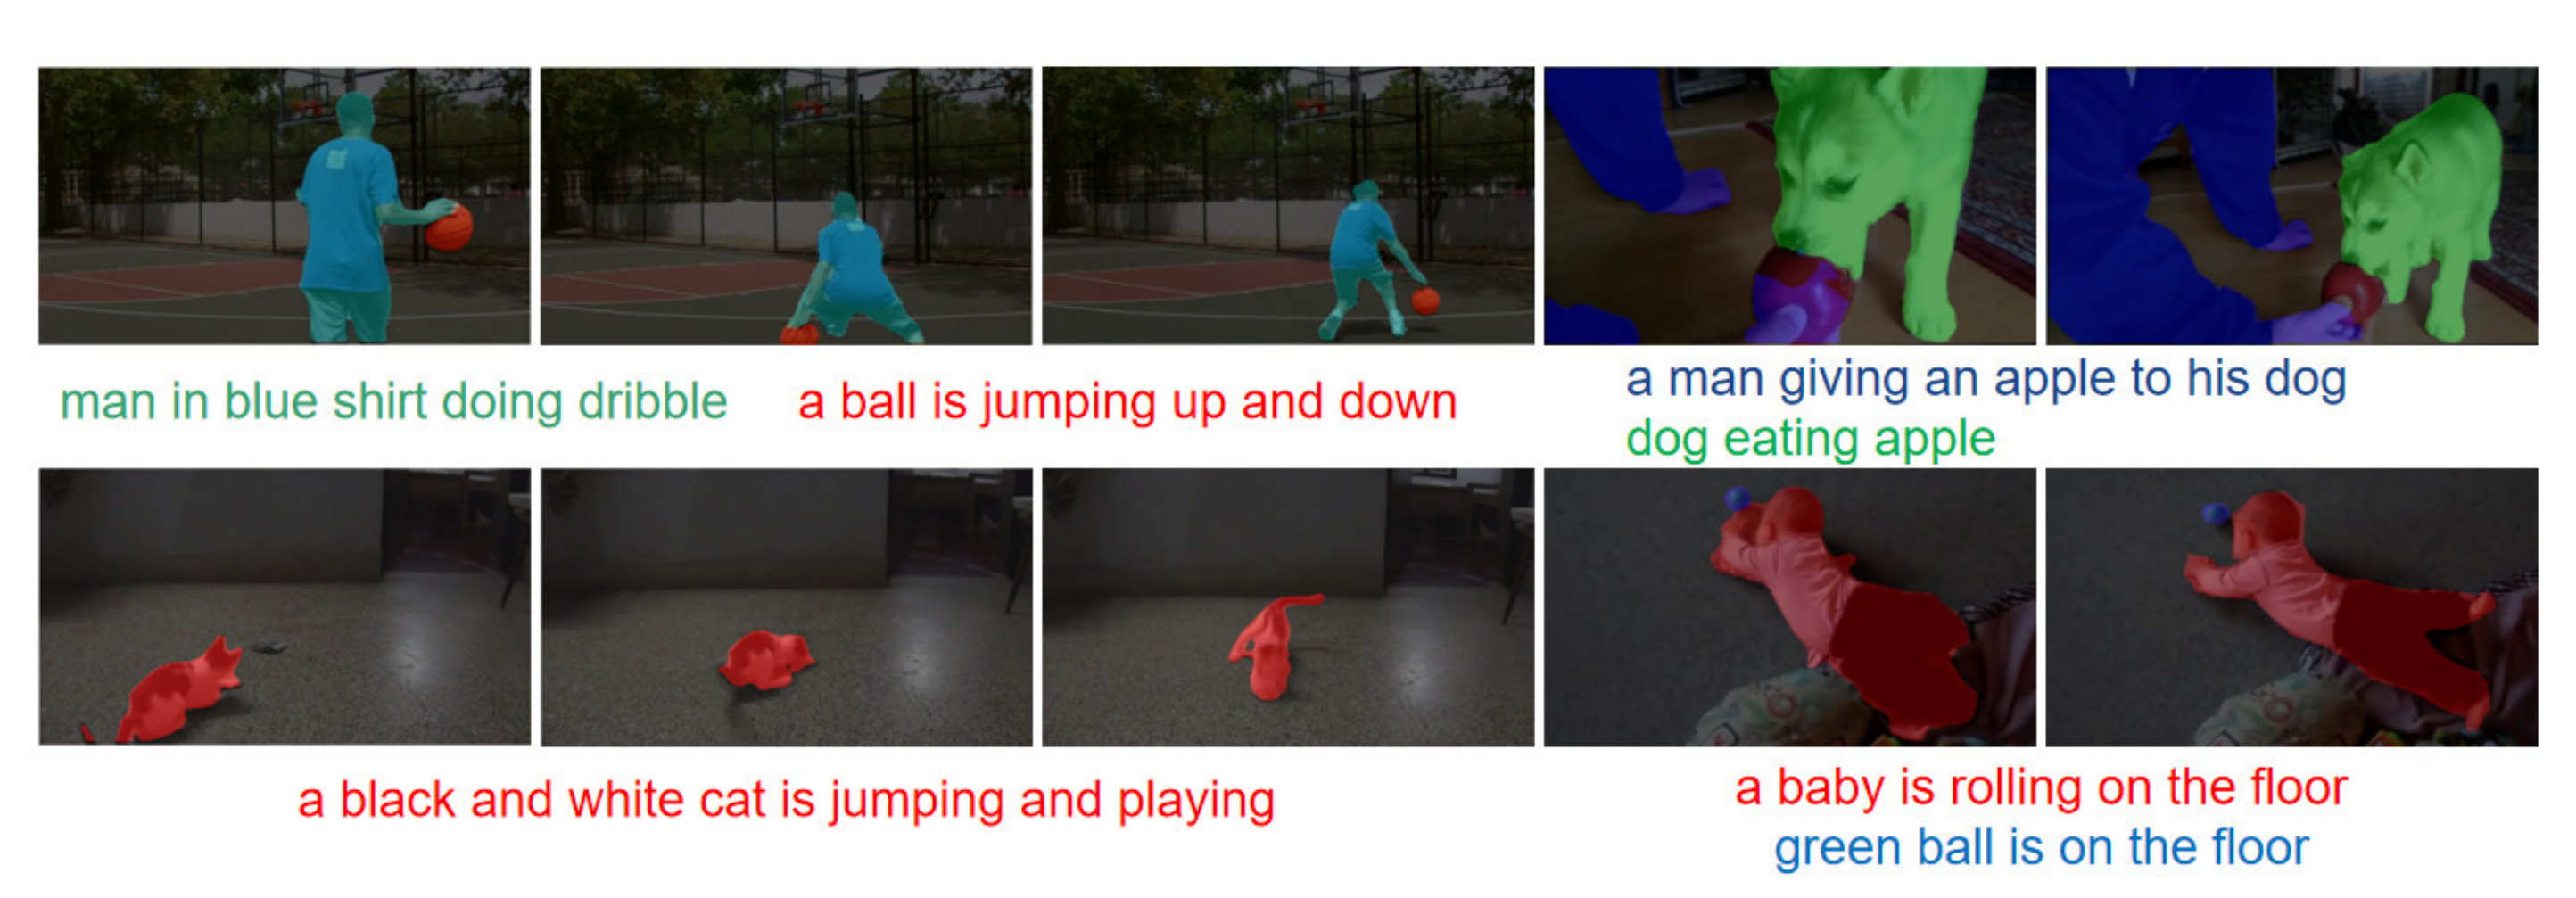}
\end{center}
\setlength{\abovecaptionskip}{-0.3cm}
\setlength{\belowcaptionskip}{-0.2cm}
   \caption{Qualitative results of LoSh across frames.}
\vspace{-6pt}
\label{fig:visualization}
\end{figure*}

\section{Additional ablation studies on LoSh-S}
In this section, we provide basic ablation studies on LoSh-S with Video-Swin-T as visual encoder and RoBERTa as linguistic encoder in terms of our proposed components.

\noindent
\textbf{Long-short text joint prediction.} Similar to Sec.~4.4 in the paper, we first present the result of LoSh-S using only the long text expressions without the short text expressions (LoSh-S w/o Sh), which is equivalent to the baseline SgMg~\cite{SgMg} with the proposed forward-backward visual consistency. The result is reported in Tab.~\ref{tab:Ablation components}: compared to LoSh-S, LoSh-S w/o Sh has a clear performance drop on mAP and IoU, \eg, -1.1 on mAP and -0.8\% on both IoU.  
We then present the result of LoSh-S without the proposed long-short cross-attention modules, \ie, LoSh-S w/o CA in Tab.~\ref{tab:Ablation components}. It shows a 0.4 decrease on mAP compared to LoSh-S.
Last, we ablate the proposed long-short predictions intersection loss $\mathcal L_{lsi}$ by presenting a variant of LoSh-S without using $\mathcal L_{lsi}$, \ie, LoSh-S w/o $\mathcal L_{lsi}$. The long-short text expressions and cross attention are still used. According to  Tab.~\ref{tab:Ablation components}, we observe a  1.3 decrease on mAP from LoSh-S to LoSh-S w/o $\mathcal L_{lsi}$. Without using $\mathcal L_{lsi}$, the model can not well align the predicted masks for the long and short text expressions.

\noindent
\textbf{Forward-backward visual consistency loss.}  We present the result of LoSh-S without using the forward-backward visual consistency loss, \ie LoSh-S w/o $\mathcal L_{fbc}$ in Tab.~\ref{tab:Ablation components}. We observe a 0.3 decrease on mAP and 0.4\% decreases on both Overall IoU and Mean IoU, compared to LoSh-S.

% \section{Alternative baseline: ReferFormer \vs enhanced LoSh-R}
% We also build our proposed LoSh on another query-based RVOS method, ReferFormer~\cite{ReferFormer}, namely LoSh-R. Since the settings of ReferFormer~\cite{ReferFormer} and SgMg~\cite{SgMg} are similar, the implementation details of LoSh-R are pretty much the same to LoSh-S (see Sec.~4.2). As demonstrated in Tab.~\ref{tab:comparison_LoShR}, LoSh-R shows consistent and significant improvements in segmentation performance on all four datasets as LoSh-M and LoSh-S in the main body of our paper.

\section{Additional qualitative results}
\noindent\textbf{Qualitative results for long-short text predictions.}
Compared with the long text expressions, the short ones are more generic expressions which normally contain only the appearance-related information of the subjects. Recalling to Sec.~4.2, there exists a few cases (approximately 10\% in RVOS datasets) in which they refer to multiple instances in video clips. We visualize the respective mask predictions corresponding to long and short text expressions in these cases. According to Fig.~\ref{fig:visualization_appendix}, the mask prediction of LoSh using the short text expression tends to cover a broader potential area in the input video compared to that generated using the long text expression. Although  the short text expressions refer to more instances in these examples, our LoSh can still generate reasonable mask predictions for them.

\noindent\textbf{Qualitative results across frames.} We show the qualitative results of LoSh across frames in Fig.~\ref{fig:visualization}.  Our model can successfully segment the target instances corresponding to the input text expressions in challenging scenarios (\eg, partial disappearance in the camera, high-speed and frequent movement, variety of poses, occlusion).

% Remove this part as our discussion.
% \subsection{LoSh without mask annotations for short text expressions.}
% Recalling Sec.~\ref{implementation}, mask annotations for short text expressions can be easily obtained. We also conduct experiments on LoSh without using the above ground truth masks (GT) for short text expressions during training. The performance degradation of the model  (around 0.25 on mAP) is acceptable when only mask annotations for full text expressions are accessible. We suggest the reasons are that 1) it is rare for a short text expression to refer to multiple instances according to our statistical analysis; 2) the proposed long-short cross-attention module can still strengthen $\mathcal F^\text{l}$ by important appearance-related information in $\mathcal F^\text{s}$ with GT for full text expressions; 3) multiple instances might be predicted by the short text expression once the mentioned rare cases happen. GT for full text expression however drives the optimization towards the referred target instance.
% As a result of both the short expression guidance and the single GT constraint, predictions on other instances might become less precise while prediction on the target instance is still ensured with good quality. \linfeng{Move 'LoSh without short text ground truth' here. And introduce two new reasons (1,2) besides the reason in Rebuttal.}

\end{appendix}
% \clearpage
